# Supplementary material for: ASER: A Large-scale Eventuality Knowledge Graph
Source: arXiv:1905.00270 source file (2020-01-25)
Supplement: Supplementary file 1 [file appendix.tex]

\clearpage

\appendix

% \section{Inference with Eventuality Information}\label{sec:appendix-inference-with-eventuality}
% One example of using the eventuality statistical information to do the inference is as following: given one sentence `The dog is chasing the cat, suddenly it barks.' and our job here is to understand which one does `it' refers to.
% To solve that problem, our system firstly extract two eventualities `dog is chasing cat' and `it barks'. As the pronoun `it' is not that informative in this example, we replace it with the two candidates `dog' and `cat' to generate two pseudo-eventualities. 
% Using these four eventualities as input, we can get their statistic information from ASER KG and it turns out that `the dog barks' appears 12,247 times while `the cat barks' only appears zero times.
% As a result, the system can understand compared with cats, dogs are more likely to bark and it can thus make the correct prediction.

\section{Pseudo-code of Eventuality Extraction}
\label{sec:appendix-event-extraction}
The eventuality extraction algorithm is shown in Algorithm~\ref{algorithm:eventuality-extraction}.

\begin{algorithm}[h]\caption{Eventuality Extraction with One Pattern $P_i$}\label{algorithm:eventuality-extraction}
			\begin{flushleft}
			\textbf{INPUT:} Parsed dependency graph $D$, center verb $v$. Positive dependency edges $P_i^p$, optional edges $P_i^o$, and negative edges $P_i^n$.
            
            \textbf{OUTPUT:} Extracted eventuality $E$.
             \end{flushleft}
            \begin{algorithmic}[1]
            \State Initialize eventuality $E$.
            \For{Each connection $d$ (a relation and the associated word) in positive dependency edges $P_i^p$}  
                \If{Find $d$ in $D$}
                    \State Append $d$ in $E$.
                \Else
                	\State Return NULL.
                \EndIf 
            \EndFor
            \For{Each connection $d$ in optional dependency edges $P_i^o$}  
                \If{Find $d$ in $D$}
                      \State Append $d$ in $E$.
                \EndIf 
            \EndFor
            \For{Each connection $d$ in negative dependency edges $P_i^n$}  
               \If{Find $d$ in $D$}
                   \State Return NULL.
               \EndIf 
            \EndFor
            \State Return $E$
            \end{algorithmic}
            
        \end{algorithm}
        \vspace{-0.15in}
\section{\revisehm{ASER Construction} Details}\label{sec:appendix-bootstrapping-details}

For preprocessing, we first parse all the raw corpora with the Stanford Dependency parser, which costs eight days with two 12-core Intel Xeon Gold 5118 CPUs. After that, We extract eventualities, build the training instance set, and extract seed relations, which costs two days with the same CPUs.
% In the section, we introduce the hyper-parameters as well as some implementation details used in the neural bootstrapping.
For bootstrapping, 
% we have high-quality relations extracted by our seed rules. We set a reasonable initial threshold $\tau_0=0.99$. As the bootstrapping continues, the quality is going down. Hence, we use the annealing strategy to increase the threshold, e.g. $\tau_1=0.9902$, $\tau_5=0.9950$, $\tau_{10}=0.9999$. Bootstrapping ends after 10 epochs.
Adam optimizer \cite{kingma:adam} is used and the initial learning rate is 0.001. The batch size is 512. We use GloVe as the pre-trained word embeddings. The dropout rate is 0.2 to prevent overfitting. The hidden sizes of LSTMs are 256 and the hidden size of the two-layer feed forward network with ReLU is 512. 
As relation types belonging to different categories could both exist in one training instance, in each bootstrapping iteration, four different classifiers are trained corresponding to four categories (\textbf{Temporal}, \textbf{Contingency}, \textbf{Comparison}, \textbf{Temporal}).
Each classifier predicts the types belong to that category or `None' of each instance. Therefore, classifiers do not influence each other so that they can be processed in parallel. Each iteration using ASER (core) takes around one hour with the same CPUs and four TITAN X GPUs. We spend around eight hours predicting ASER (full) with the learned classifier in the 10th iteration.

\section{Distribution of Eventualities}\label{sec:appendix-eventuality-distribution}
\begin{figure}[t]
    \centering
    \includegraphics[width=\linewidth]{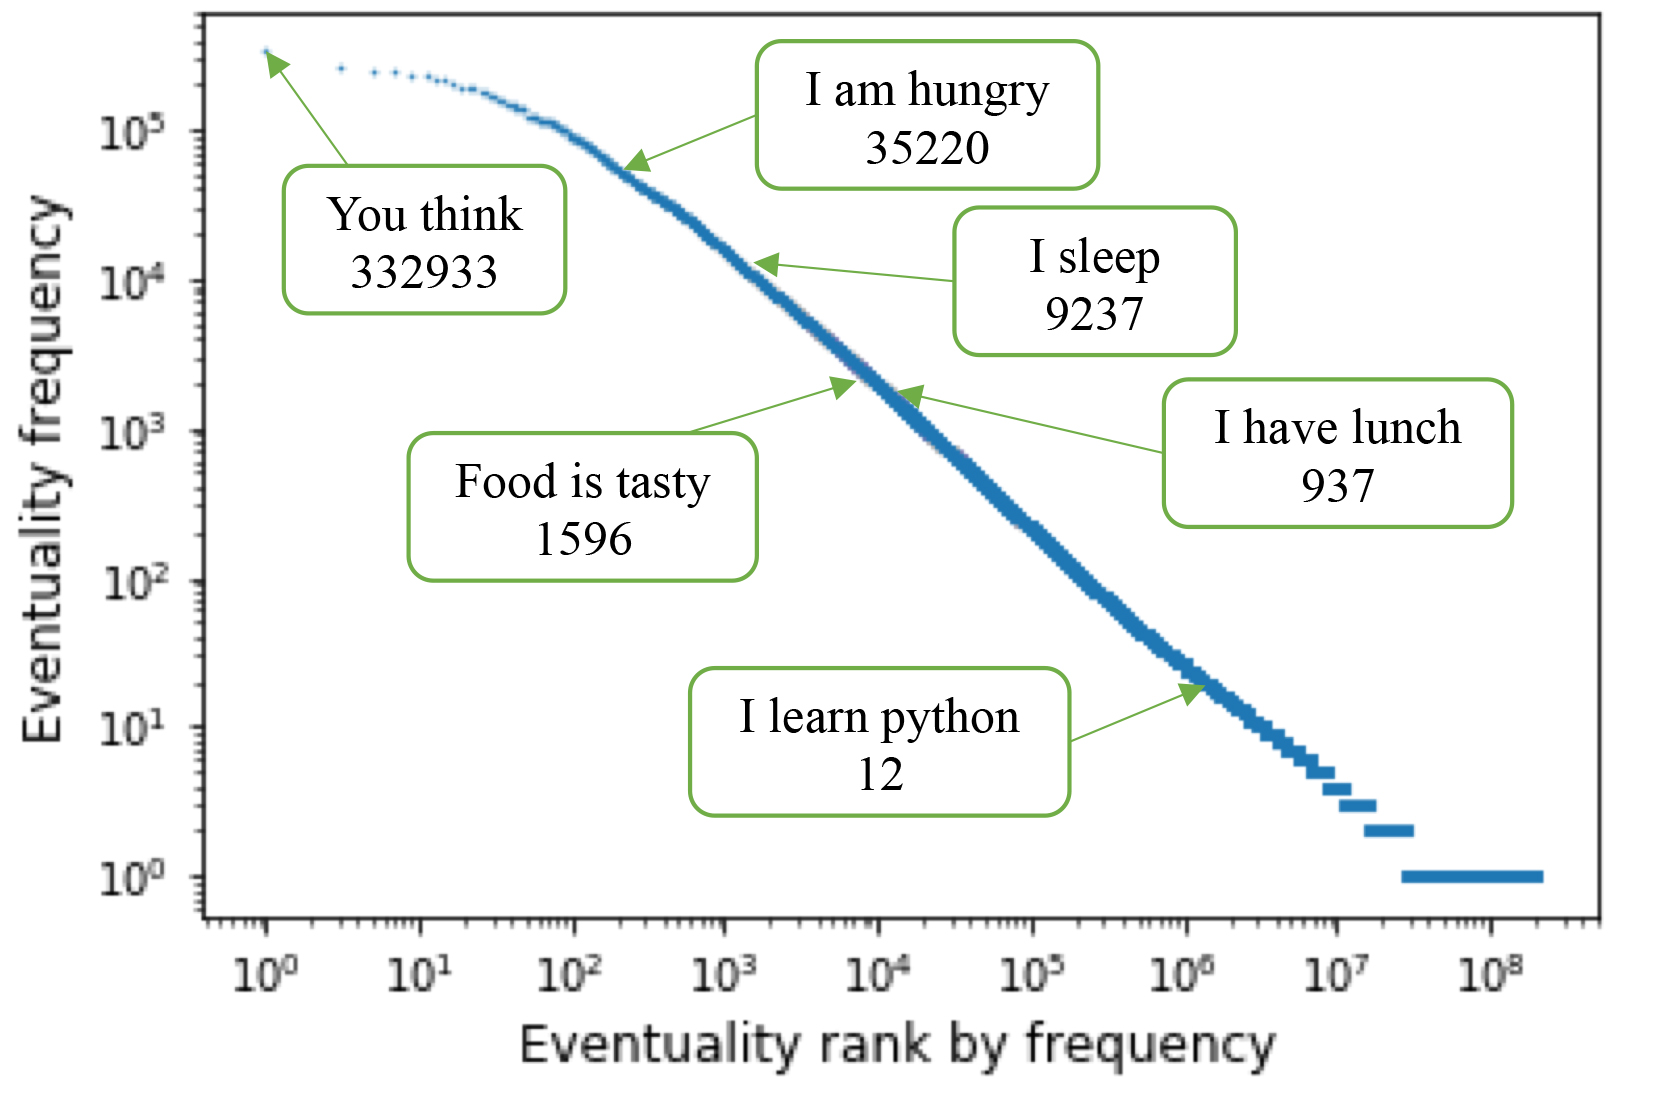}
    \vspace{-0.1in}
    \caption{\small Distribution of eventualities by their frequencies. Sampled eventualities are shown along with their frequencies.}
    \label{fig:dist_eventualities}
    \vspace{-0.2in}
\end{figure}

The distribution of extracted eventualities is shown in Figure~\ref{fig:dist_eventualities}.
In general, the distribution of eventualities follows the Zipf's law, where only a few eventualities appear many times while the majority of eventualities appear only a few times.

To better illustrate the distribution of eventualities, we also show several representative eventualities along with their frequencies and we have two observations.
First, eventualities which can be used in general cases, like `You think', appear much more times than other eventualities.
Second, eventualities contained in ASER are more related to our daily life like `Food is tasty' or `I sleep' rather than domain-specific ones such as `I learn python'.
%Incorporating more \reviseyq{domain-specific} knowledge is one of our important future work.

\section{Experiment Implementation Details}
\subsection{Winograd Schema Challenge}
\label{sec:appendix-wino}

% \subsection{Implementation} 
% \label{sec:appendix-wino-implementation}

To demonstrate the effectiveness of ASER, we try to solve Winograd questions using simple inference based on ASER.
For each question sentence $s$, we first extract eventualities with the same method introduced in Section~\ref{sec:eventuality-extraction} and then select eventualities $E_{n_1}$, $E_{n_2}$, and $E_p$ that contain candidates nouns $n_1$/$n_2$ and the target pronoun $p$ respectively. 
We then replace $n_1$, $n_2$, and $p$ with placeholder $X$, $Y$, and $P$,  and hence generate the pseudo-eventualities $E_{n_1}^\prime$, $E_{n_2}^\prime$, and $E_p^\prime$.
After that, if we can find the seed connectives in Table~\ref{tab:seed-pattern} between any two eventualities, we use the corresponding relation type as relation type $T$. Otherwise, we use \textit{Co\_Occurrence} as the relation type.  
To evaluate the candidate, we first replace the placeholder $P$ in $E_p^\prime$ with the corresponding placeholders $X$ or $Y$ and then use the following equation to define its overall plausibility score:
\begin{equation}
    F(n, p) = ASER_R(E_n^\prime, E_p^\prime),
\end{equation}
where $ASER_R(E_n, E_p)$ indicates the number of edges in ASER that can support that there exist one typed $T$ relation between the eventuality pairs $E_n^\prime$ and $E_p^\prime$.
For each edge ($E_h$, $T$, $E_t$) in ASER, if it can fit the following three requirements:
\begin{enumerate}
    \item $E_h$ = $E_n^\prime$ other than the words in the place holder positions.
    \item $E_t$ = $E_p^\prime$ other than the words in the place holder positions.
    \item Assume the word in the placeholder positions of $E_h$ and $E_t$ are $w_h$ and $w_t$ respectively, $w_h$ has to be same as $w_t$.
\end{enumerate}
we consider that edge as a valid edge to support the observed eventuality pair.
If any of $E_n$ and $E_p$ cannot be extracted with our patterns, we will assign 0 to $F(n, p)$.
We then predict the candidate with the higher score to be the correct reference. If both of them have the same score (including 0), we will make no prediction.

% \subsection{Case Study}
% \label{sec:appendix-wino-case}
\begin{figure}[t]
    \centering
    \includegraphics[width=\linewidth]{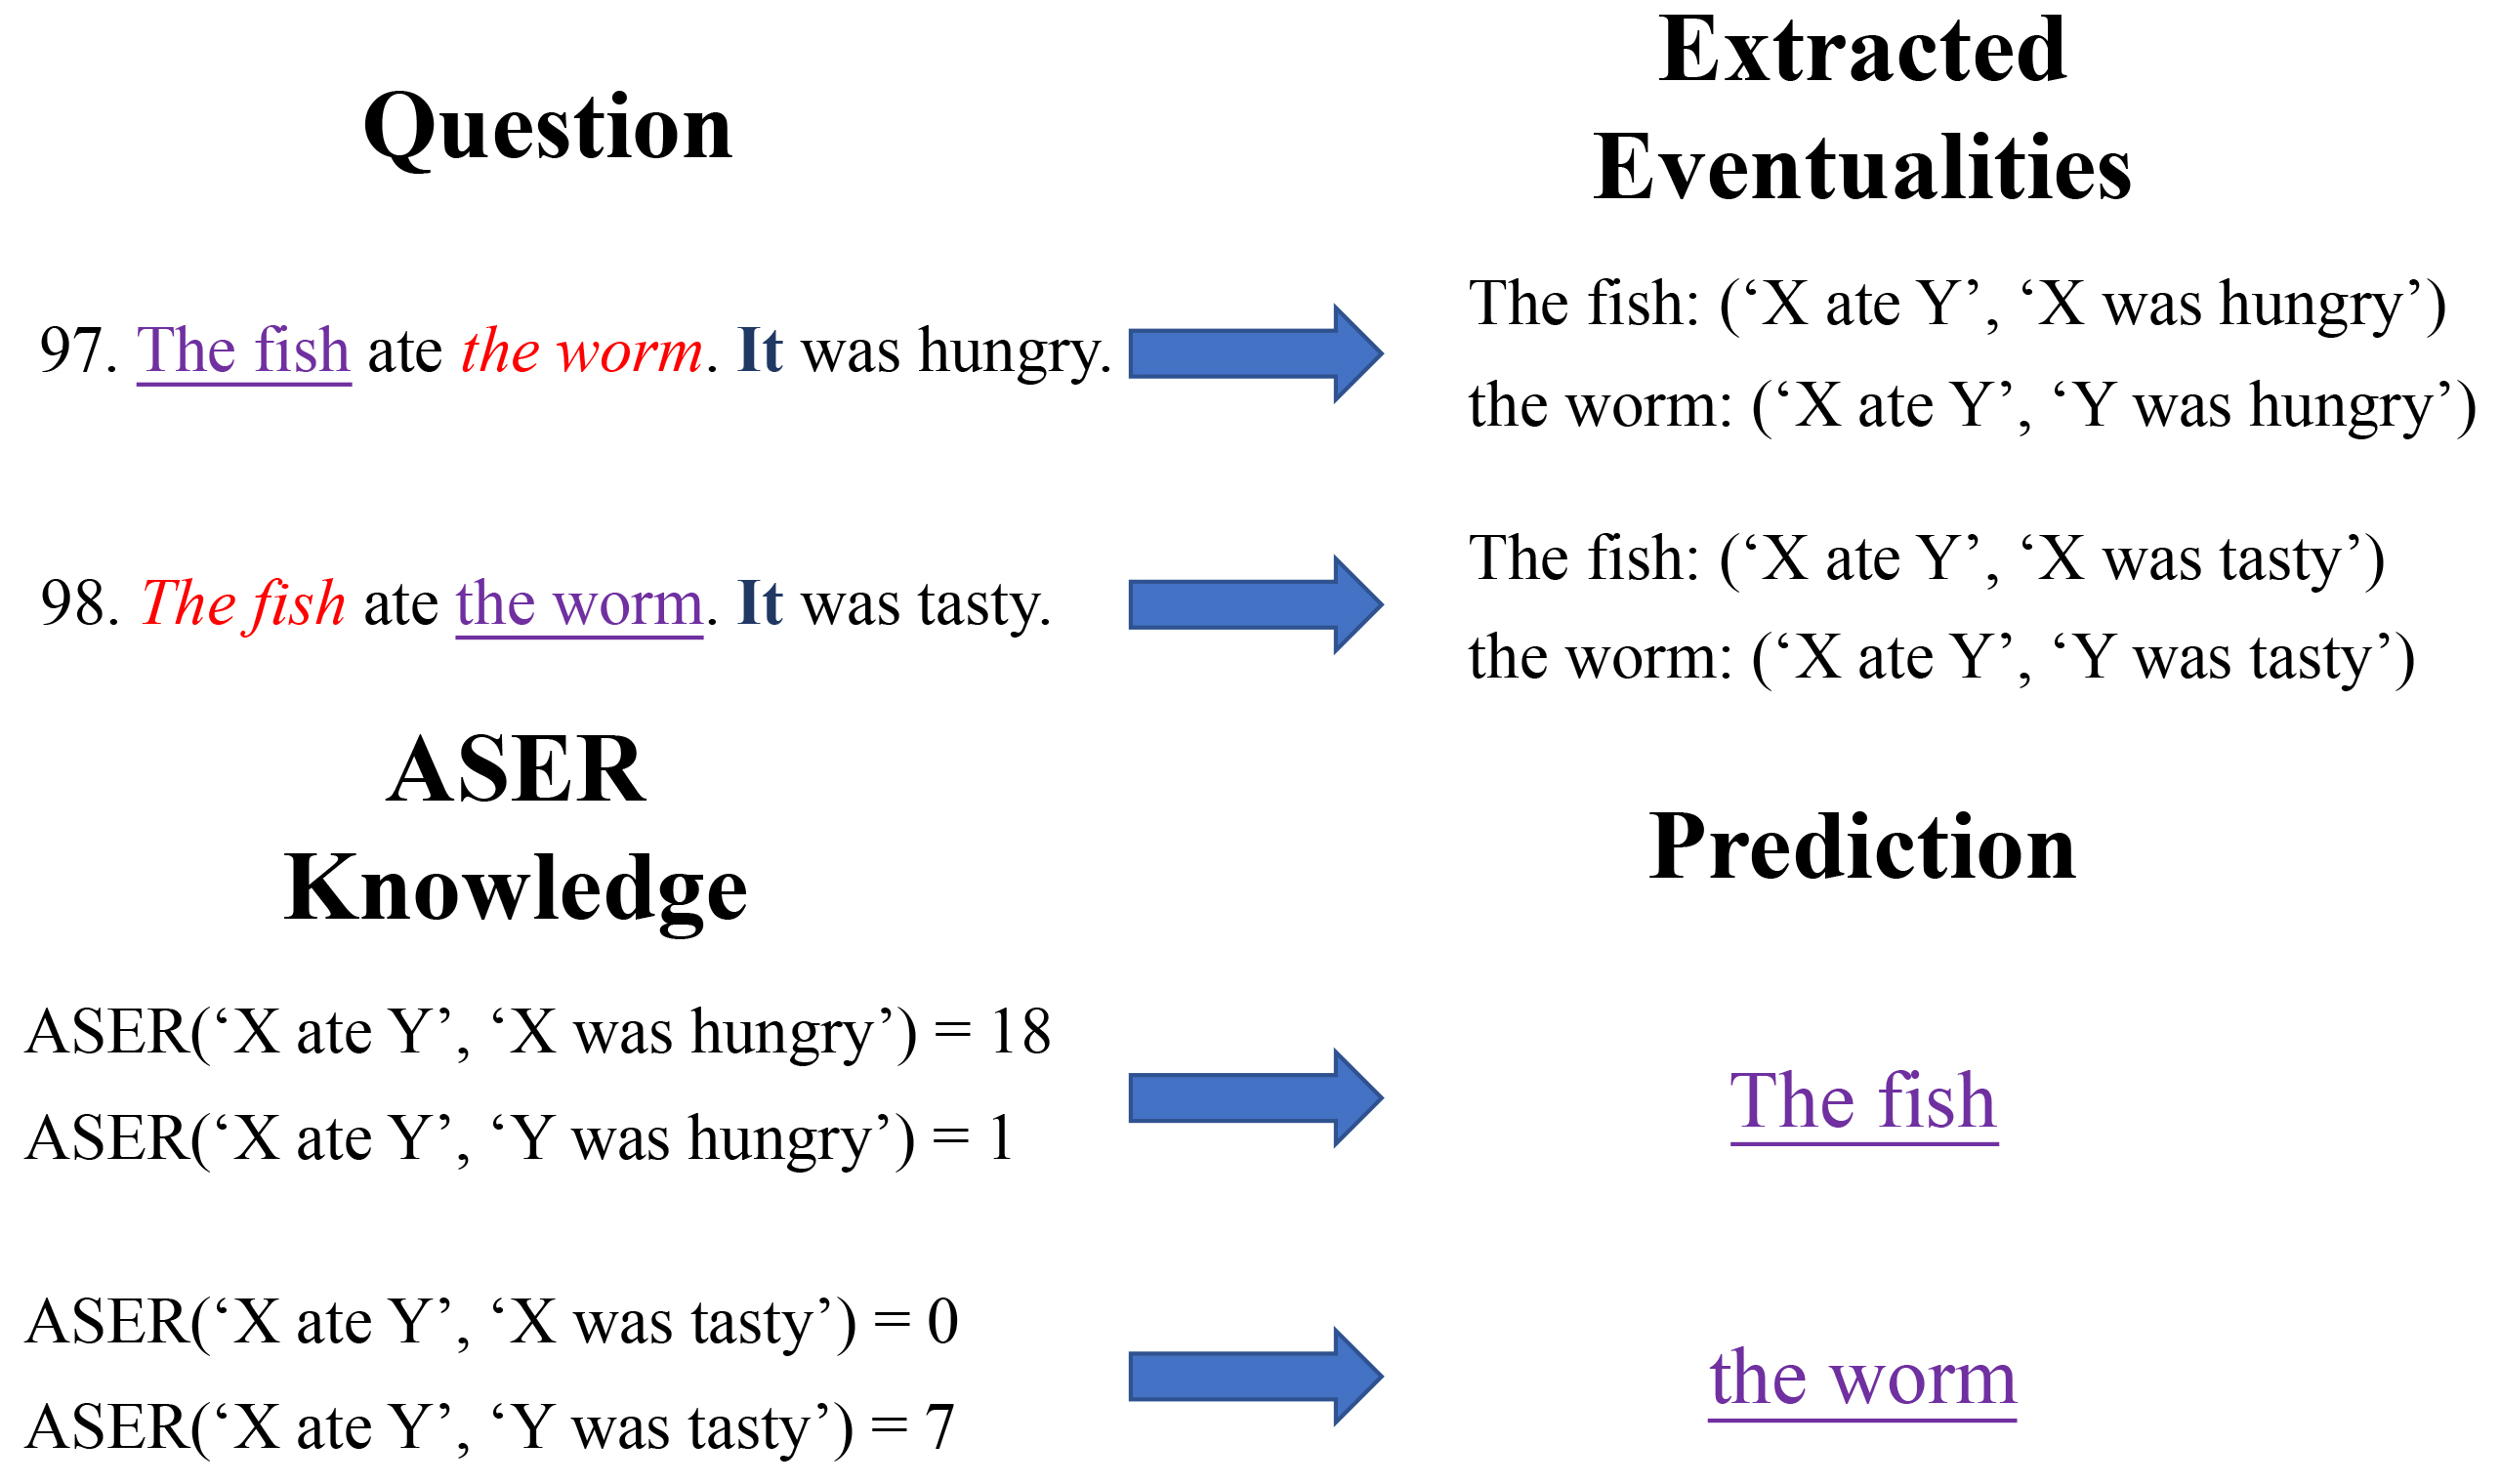}
    \caption{\small Example of using ASER to solve Winograd questions. The number before questions are the original question ID in the Winograd dataset. Correct answer and the other candidate are labeled with purple underline and red italic font respectively. }
    \label{fig:wino_case_study}
    \vspace{-0.2in}
\end{figure}

% On the other hand, the proposed model built on ASER can better predict the correct reference due to its capability of contained commonsense knowledge in relation between eventualities.
As shown in Figure~\ref{fig:wino_case_study}, our model can correctly resolve `it' to `fish' in question 97, because 18 edges in ASER support that the subject of `eat' should be `hungry', while only one edge supports the object of `eat' should be `hungry'. Similarly, our model can correctly resolve `it' to `the worm' in question 98, because seven edges in ASER support that the object of `eat' should be `tasty' while no edge supports that the subject of `eat' should be `tasty'.

\subsection{Dialogue Generation}\label{sec:appendix-dialog}

In this section, we introduce how we incorporate knowledge about eventualities into a memory module and the eventuality matching case study.

For each conversation pair, which contains one post and one response, we first extract eventualities\footnote{Different KGs have different definitions of eventuality. Hence, we use different formats to extract eventuality based on their original settings (OMCS uses strings to represent eventualities, KnowlyWood uses a verb-object pair to define eventualities, and ASER uses dependency graphs to represent eventualities).} from post $p$. Then we get eventuality set $\E_p$, which contains $m$ eventualities $\{E_1, E_2, ..., E_m\}$. For each $E_i \in \E_p$, we search it in the KG and retrieval all related edges, which are represented as triplets.
% Assume $e_i$ is connected with $m_i$ eventualities in knowledge base, we denote them as $\{(e_{i,1}, r_{i,1}), (e_{i,2}, r_{i,2}), ..., (e_{i,m_i}, r_{i,m_i})\}$, where $e_{i,j}$ represents the $j^{th}$ eventuality connected with $e_i$ in ASER and $r_{i,j}$ is the corresponding relation between these two events\footnote{If there are multiple relations between two events, we will treat the eventuality-relation pair separately.}. 
% Then we can get a list of 
% triples $\{(e_{1}, r_{1, 1}, e_{1, 1}), ..., (e_{1}, r_{1, m_1}, e_{1, m_1}), ..., (e_{k}, r_{k, 1}, e_{k, 1}), \\ ..., (e_{k}, r_{k, m_k}, e_{k, m_k})\}$
For each triplet $(E_{src}, R, E_{tgt})$, where $E_{src}$ is the eventuality we extract from the post, $E_{tgt}$ is the retreivaled related eventuality, and $R$ is the relation type between them, we represent it as a concatenation of four vectors $\widetilde v_k = [v_{tri} | v_{src} | v_{rel} | v_{tgt}]$, where $v_{tri}$, $v_{src}$, $v_{rel}$, and $v_{tgt}$ are the embeddings of the triplets, $R$, $E_{src}$, and $E_{tgt}$ respectively. All of them are set to be trainable.
% Assuming we have $K$ triples, then we can represent external knowledge as memory $\{\widetilde M_k\}_{k=1}^K$.
We group the representations of all triplets as a memory $\widetilde M$.
We use cross-entropy as the loss and Adam \cite{kingma:adam} with the initial learning rate of 0.005 to update all parameters, which are initialized randomly.
% The dimension of encoder biGRU hidden state is 256 for each direction, and 512 for the decoder GRU, we use two layer GRU for both encoder and decoder. 
We use the 256-dimension two-layer biGRU as the encoder and the 512-dimension two-layer GRU as the decoder.
The word embedding size is set to 300 and the embedding sizes of $v_{tri}$, $v_{src}$, $v_{rel}$, and $v_{tgt}$ are all 128.  All the models are trained up to 20 epochs and the best models are selected based on the dev set. Dropout is set to be 0.1. In the inference stage, the beam search size is set to be five.

\begin{table}[t]
    \centering
    \caption{\small Statistics of the dialogue dataset. \# Covered pairs means the number of conversation pairs, whose eventualities can be covered by the corresponding KG. coverage rate means the percentage of such pairs. And \# Unique matched events means the number of unique matched eventualities in the KG.}\label{tab:dialog_statistics}
    \vspace{-0.05in}
    {\footnotesize
    \begin{tabular}{c|cc|c}
    \toprule
        KG  & \# Covered pairs & Coverage rate & \# Unique matched events  \\
    \midrule
        OMCS & 7,246  & 24.04\% & 1,195 \\
        KnowlyWood & 17,183 & 57.00\% & 30,036\\
        \midrule
        ASER       & 20,494 & 67.98\% & 9,511\\
        % \# Events & & & \\
        % \# R. Types & \\
        
         \bottomrule
    \end{tabular}
    }
    \vspace{-0.1in}
\end{table}

\begin{table}[t]
\caption{\small Eventuality matching example.}
\vspace{-0.1in}
{\footnotesize
	\begin{tabular}{c|c}
		\toprule
		Post & 	I should eat some food . \\
		\midrule
		Response & Yeah, you must be hungry. Do you like to eat some beaf? \\
		\midrule
		\multirow{2}{*}{OMCS} & `eat food', MotivatedByGoal, `you are hungry' \\   
		 & `eat food', HasPrerequisite, `open your mouth' \\
		\midrule
		\multirow{4}{*}{KnowlyWood} & (eat,food), next, (keep, eating) \\   
		 & (eat,food), next, (enjoy, taste) \\
		 & (eat,food), next, (stick, wasp) \\
		 & ... \\
		\midrule
		\multirow{4}{*}{ASER} & i eat food [s-v-o], Conjunction, beef is good [s-be-a] \\ 
		 & i eat food [s-v-o], Condition, i am hungry [s-be-a] \\
		 & i eat food [s-v-o], Concession, i take picture [s-v-o] \\
		 & ... \\
		\bottomrule
	\end{tabular}
	\vspace{-0.15in}
	}
	\label{tab:dialog_sample}
\end{table}

The detailed statistics about the coverages of different KGs are shown in Table~\ref{tab:dialog_statistics}. The number of covered conversation pairs, the percentage of such pairs, and the number of unique covered eventualities of each KG are reported. 
The statistics show that OMCS can only cover a very small portion of the questions due to its relatively small size and ASER covers the most conversation pairs.
We also notice that compared with ASER, Knowlywood can cover more eventualities in fewer conversation pairs. 
The reason behind is that the definition of eventuality is different. 
In Knowlywood, each eventuality is represented with two words (verb+object), which may not be semantically complete but can be more easily found in the text. In ASER, we require the matched eventualities to be semantically complete, each of which typically contains 3-5 words. This makes them more difficult to be matched. 
Nonetheless, as ASER is extracted from different resources, it can cover the topics in more conversation pairs.

One example is shown  in Table~\ref{tab:dialog_sample}. After getting the post `I should eat some food', we extract the contained eventuality `eat food', `eat food', and `I eat food' for the three KGs respectively, and then find the related eventualities in KGs to generate the response.
By retrieving from OMCS, we know that `eat food' can be motivated by `you are hungry' and has the prerequisite that we have to open our mouth. 
Similarly, by retrieving from KnowlyWood, we know that we often `keep eating', `enjoy taste', or `stick swap' after `eat food'.
By retrieving from ASER, we know that `I eat food' and `beef is good' can happen at the same time, and eating food often has the condition of being hungry.

In general, the OMCS is accurate and correct, because they are generated by humans. However, their small scale limits their usage. 
KnowlyWood has a better scale, but its semantically incomplete definition of eventualities also limits the usage.
As a comparison, ASER leverages carefully designed patterns to make sure the semantic completeness of extracted eventualities and uses a neural bootstrapping model to automatically learn relations between eventualities from large unlabeled corpus. Thus, it can provide a larger scale and higher quality eventuality knowledge.

% \section{\revisexin{APIs}}\label{sec:appendix-APIs}
% \begin{figure*}[t]
%     \centering
%     \includegraphics[width=\linewidth]{image/API.png}
%     \caption{\small Simple APIs of ASER.}
%     \label{fig:API}
% \end{figure*}
% Some simple APIs of ASER are also illustrated. The first line is to load our package. We use the KG\_Connection to load the core KG in the second line. We provides three different modes, including insert, cache and memory. The insert mode allows to update the KG. The memory mode   fetches all data from the database and store them in memory to speed up retrievals afterwards. The cache mode retrieves and caches requested rows from the database only when users need some data that memory misses.
% The third line outputs the schema of the EVENTUALITIES table and the next line prints the information of 'I learn python'. The fifth line shows the schema of the RELATIONS table and the last line provides the relations between 'I am tired' and 'I sleep'. It's worth noting that the \textit{Result} with a probability of 0.9970 is learned via bootstrapping, because all probabilities of relations extracted using pattern based methods must equal 1.
